# Supplementary material for: Exponentially Convergent Direct Adaptive Pole Placement Control of Plants with Unmatched Uncertainty under FE Condition
Source: arXiv:2201.01228 ancillary file (2022-04-11)
Supplement: Supplementary file 1 [file supp_v2.pdf]

# Supplement to ”Exponentially Convergent Direct Adaptive Pole Placement Control of Plants with Unmatched Uncertainty under FE Condition” Submitted to IEEE Control Systems Letters

A. Glushchenko, *Member, IEEE*, and K. Lastochkin

**Abstract**

This article is a supplementary material for ”Exponentially Convergent Direct Adaptive Pole Placement Control of Plants with Unmatched Uncertainty under FE Condition” submitted to IEEE Control Systems Letters by the same authors. It provides more details on how to obtain the parametrization (15) and the equation (A13) and is being referred to in appropriate places.

## I. Explanation on how to obtain parametrization (15) in the manuscript

First of all, let the equation (5) from the manuscript be presented:

$$\dot{x}(t) = \theta_{AB}^{\mathrm{T}}\Phi(t),\, \theta_{AB}^{\mathrm{T}} = \begin{bmatrix} A & B \end{bmatrix},\, \Phi(t) = \begin{bmatrix} x^{\mathrm{T}}(t) & u(t) \end{bmatrix}^{\mathrm{T}}, \tag{S1}$$

where $\Phi(t) \in \mathbb{R}^{n+1}$ is the measurable regressor, $\theta_{AB}^{\mathrm{T}} \in \mathbb{R}^{n\times(n+1)}$ is the matrix of the unknown parameters.

Despite the fact that $\dot{x}(t)$ is unmeasurable, let the following stable linear filters be introduced:

$$\begin{array}{c} \dot{\overline{\mu}}(t) = -l\overline{\mu}(t) + \dot{x}(t),\, \overline{\mu}(0) = 0_n, \\ \dot{\overline{\Phi}}(t) = -l\overline{\Phi}(t) + \Phi(t),\, \overline{\Phi}(0) = 0_{n+1}, \end{array} \tag{S2}$$

where $l > 0$ is the filter constant.

According to [1], the function $\overline{\mu} > 0$ could be calculated without the value of $\dot{x}(t)$ as follows:

$$\begin{array}{c} \overline{\mu}(t) = e^{-lt}\overline{\mu}(0) + x(t) - e^{-lt}x(0) - l\overline{x}(t) + le^{-lt}\overline{x}(0) = \\ = x(t) - e^{-lt}x(0) - l\overline{x}(t), \end{array} \tag{S3}$$

where $\overline{x}(t)$ is the element of the vector $\overline{\Phi}(t)$.

Considering the filtration (S2) and the fact that the initial conditions in (5) in the manuscript are unknown, (S1) is rewritten as:

$$\begin{array}{c} \overline{\mu}(t) = \theta_{AB}^{\mathrm{T}}\overline{\Phi}(t) \Rightarrow \\ \Rightarrow x(t) - e^{-lt}x(0) - l\overline{x}(t) = \theta_{AB}^{\mathrm{T}}\overline{\Phi}(t) \Rightarrow \\ \Rightarrow x(t) - l\overline{x}(t) = \theta_{AB}^{\mathrm{T}}\overline{\Phi}(t) + e^{-lt}x(0) \Rightarrow \\ \Rightarrow \overline{z}(t) = x(t) - l\overline{x}(t) = \theta_{AB}^{\mathrm{T}}\overline{\Phi}(t) + e^{-lt}x(0) = \overline{\theta}_{AB}^{\mathrm{T}}\overline{\varphi}(t), \\ \overline{\varphi}(t) = \begin{bmatrix} \overline{\Phi}^{\mathrm{T}}(t) & e^{-lt} \end{bmatrix}^{\mathrm{T}},\, \overline{\theta}_{AB}^{\mathrm{T}} = \begin{bmatrix} A & B & x(0) \end{bmatrix}, \end{array} \tag{S4}$$

where $\overline{z}(t)$ is the measurable function, $\overline{\varphi}(t) \in \mathbb{R}^{n+2}$ is the measurable regressor, $\overline{\theta}_{AB}^{\mathrm{T}} \in \mathbb{R}^{n\times(n+2)}$ is the augmented vector of the unknown parameters.

## II. Explanation on how to obtain the equation (A13) in the manuscript

Considering that $adj\left\{\overline{\Delta}(t)\right\}\overline{\Delta}(t) = det\left\{\overline{\Delta}(t)\right\}I_{(n+1)\times(n+1)}$, the equation (A12) in the manuscript is multiplied by $adj\left\{\overline{\Delta}(t)\right\}$ to obtain:

$$\begin{array}{c} Y(t) := adj\left\{\overline{\Delta}(t)\right\}\overline{Y}(t), \\ \Delta(t) := det\left\{\overline{\Delta}(t)\right\} = \Delta_x(t)\,\Delta_r(t). \end{array} \tag{S5}$$

This research was financially supported by the Presidential Fund of Russia (project MD-1787.2022.4).
Anton Glushchenko is with V.A. Trapeznikov Institute of Control Sciences of RAS, Moscow, Russia (e-mail: aiglush@ipu.ru).
Konstantin Lastochkin is with V.A. Trapeznikov Institute of Control Sciences of RAS, Moscow, Russia (e-mail: lastconst@ipu.ru).

**Step 1.** The regressor $\Delta_x(t)$ is to be expressed in terms $\varphi(t)$ and some unknown constants $C_1$, $C_2$, $C_3$. For that, first of all, the definitions of $\overline{\Delta}_x(t)$ (from (A4) in the manuscript) and $Y_M^{\rm T}(t)$ (from (A3) in the manuscript) are taken into consideration:

$$\Delta_x(t) := det\left\{\overline{\Delta}_x(t)\right\} = det\left\{Y_M^{\rm T}(t)\right\} = det\left\{\Delta_M(t)\, M^{\rm T}\right\}. \tag{S6}$$

The definition of $\Delta_M(t)$ from (A2) in the manuscript is substituted into (S6), and the properties $det\{c\Xi\} = c^n det\{\Xi\}$, $det\{\Xi\} = det\left\{\Xi^{\rm T}\right\}$ (where $c \in \mathbb{R}$ and $\Xi \in \mathbb{R}^{n\times n}$) are applied to obtain:

$$\Delta_x(t) = \Delta_M^n(t)\, det\{M\} = det\{\overline{\Delta}_M(t)\}^n det\{M\}. \tag{S7}$$

The definition of $\overline{\Delta}_M(t)$ from (A1) in the manuscript is substituted into (S7):

$$\begin{gathered}\Delta_x(t) = \left(det\left\{-I_{n\times n}\otimes z_A(t) + \varphi(t)\,\Gamma^{\rm T}\otimes I_{n\times n}\right\}\right)^n det\{M\} = \\ = \varphi^{n^3}(t)\left(det\left\{-I_{n\times n}\otimes A + \Gamma^{\rm T}\otimes I_{n\times n}\right\}\right)^n det\{M\} = C_1^n C_2 \varphi^{n^3}(t), \\ C_1 := det\left\{-I_{n\times n}\otimes A + \Gamma^{\rm T}\otimes I_{n\times n}\right\},\ C_2 := det\{M\}.\end{gathered} \tag{S8}$$

**Step 2.** Then the regressor $\Delta_r(t)$ is to be expressed in terms $\varphi(t)$ and the same unknown constants $C_1$, $C_2$, $C_3$. For that, first of all, the definitions of $Y_M(t)$ and $Y_M^{-1}(t)$ from (A3) and (A9) in the manuscript respectively are taken into consideration:

$$\Delta_r(t) := h^{\rm T} Y_M(t)\,\Gamma^{-1} Y_{M^{-1}}(t)\, z_B(t) = \Delta_M(t)\,\Delta_{M^{-1}}(t)\,\varphi(t)\, h^{\rm T} M \Gamma^{-1} M^{-1} B \tag{S9}$$

According to (A7) in the manuscript, the equality $M\Gamma^{-1}M^{-1} = A_\Sigma^{-1}$ holds. Then the equation (S9) is rewritten as:

$$\begin{gathered}\Delta_r(t) = \Delta_M(t)\,\Delta_{M^{-1}}(t)\,\varphi(t)\, h^{\rm T} A_\Sigma^{-1} B = \Delta_M(t)\,\Delta_{M^{-1}}(t)\,\varphi(t)\, C_3, \\ C_3 := h^{\rm T} A_\Sigma^{-1} B.\end{gathered} \tag{S10}$$

The definition of $\Delta_M(t)$ from (A2) in the manuscript is substituted into (S10), and the property $det\{c\Xi\} = c^n det\{\Xi\}$ (where $c \in \mathbb{R}$ and $\Xi \in \mathbb{R}^{n\times n}$) is applied to (S10) to obtain:

$$\begin{gathered}\Delta_r(t) = det\left\{\overline{\Delta}_M(t)\right\}\Delta_{M^{-1}}(t)\,\varphi(t)\, C_3 = \\ = det\left\{-I_{n\times n}\otimes z_A(t) + \varphi(t)\,\Gamma^{\rm T}\otimes I_{n\times n}\right\}\Delta_{M^{-1}}(t)\,\varphi(t)\, C_3 = \\ = det\left\{\varphi(t)\left(-I_{n\times n}\otimes A + \Gamma^{\rm T}\otimes I_{n\times n}\right)\right\}\Delta_{M^{-1}}(t)\,\varphi(t)\, C_3 = \\ = \varphi^{n^2}(t)\, det\left\{\left(-I_{n\times n}\otimes A + \Gamma^{\rm T}\otimes I_{n\times n}\right)\right\}\Delta_{M^{-1}}(t)\,\varphi(t)\, C_3 = \\ = C_1 C_3 \Delta_{M^{-1}}(t)\,\varphi^{n^2+1}(t).\end{gathered} \tag{S11}$$

Then the definition of the regressor $\Delta_{M^{-1}}(t)$ from (A9) in the manuscript is taken into consideration, and the property $det\{c\Xi\} = c^n det\{\Xi\}$ (where $c \in \mathbb{R}$ and $\Xi \in \mathbb{R}^{n\times n}$) is applied to (S11) to obtain:

$$\begin{gathered}\Delta_r(t) = C_1 det\{Y_M(t)\}\, C_3 \varphi^{n^2+1}(t) = \\ = C_1 det\{\Delta_M(t)\, M\}\, C_3 \varphi^{n^2+1}(t) = C_1 \Delta_M^n(t)\, det\{M\}\, C_3 \varphi^{n^2+1}(t) = \\ = \Delta_M^n(t)\, C_1 C_2 C_3 \varphi^{n^2+1}(t)\end{gathered} \tag{S12}$$

Considering the definition of $\Delta_M(t)$ from (A2) in the manuscript, it is obtained similarly to (S11):

$$\begin{gathered}\Delta_r(t) = det\{\overline{\Delta}_M\}^n C_1 C_2 C_3 \varphi^{n^2+1}(t) = \\ = det\{-I_{n\times n}\otimes z_A(t) + \varphi(t)\,\Gamma^{\rm T}\otimes I_{n\times n}\}^n C_1 C_2 C_3 \varphi^{n^2+1}(t) = \\ = det\{\varphi(t)\left(-I_{n\times n}\otimes A + \Gamma^{\rm T}\otimes I_{n\times n}\right)\}^n C_1 C_2 C_3 \varphi^{n^2+1}(t) = \\ = \varphi^{n^3}(t)\, det\{-I_{n\times n}\otimes A + \Gamma^{\rm T}\otimes I_{n\times n}\}^n C_1 C_2 C_3 \varphi^{n^2+1}(t) = \\ = C_1^{n+1} C_2 C_3 \varphi^{n^3+n^2+1}(t).\end{gathered} \tag{S13}$$

**Step 3.** The obtained definitions (S8) and (S13) of $\Delta_x(t)$ and $\Delta_r(t)$ respectively are substituted into the expression of $\Delta(t)$ from (S5):

$$\begin{gathered}\Delta(t) := \Delta_x^n(t)\,\Delta_r(t) = C_1^{n^2} C_2^n \varphi^{n^4}(t)\, C_1^{n+1} C_2 C_3 \varphi^{n^3+n^2+1}(t) = \\ = C_1^{n^2+n+1} C_2^{n+1} C_3 \varphi^{n^4+n^3+n^2+1}(t).\end{gathered} \tag{S14}$$

The equation (A13) in the manuscript is obtained by combining (S5) and (S14).

***Remark S1.*** *Obtained definition of the regressor $\Delta(t)$ with the help of $\varphi(t)$ and unknown constants $C_1$, $C_2$, $C_3$ is required only to prove the implication $\varphi(t) \in {\rm FE} \Rightarrow \Delta(t) \in {\rm FE}$. When the adaptive law (21) in the manuscript is implemented, $\Delta(t)$ is calculated using measurable (according to (A1)-(A11) in the manuscript) signal $\Delta_x(t)\,\Delta_r(t)$ (the left-hand side of* (S14)*).*

*The dependence of $\Delta_x(t)$ and $\Delta_r(t)$ from measurable $z_A(t)$, $z_B(t)$, $\varphi(t)$, which are obtained in (17) in the manuscript, is written in explicit form as follows:*

$$\begin{gathered}\Delta_x(t) := \det\left\{Y_M^{\rm T}(t)\right\} = \det\left\{\left(vec^{-1}\left\{adj\left\{\overline{\Delta}_M(t)\right\}\overline{Y}_M(t)\right\}\right)^{\rm T}\right\} = \\ = \det\left\{\left(vec^{-1}\left\{adj\left\{-I_{n\times n}\otimes z_A(t) + \varphi(t)\,\Gamma^{\rm T}\otimes I_{n\times n}\right\} vec\left(z_B(t)\, h^{\rm T}\right)\right\}\right)^{\rm T}\right\},\end{gathered} \tag{S15}$$

$$\begin{gathered}\Delta_r(t) := h^{\mathrm{T}} Y_M(t)\,\Gamma^{-1} Y_{M^{-1}}(t)\, z_B(t) = h^{\mathrm{T}}\left(vec^{-1}\left\{adj\left\{\overline{\Delta}_M(t)\right\}\overline{Y}_M(t)\right\}\right)\Gamma^{-1} Y_{M^{-1}}(t)\, z_B(t) = \\ = h^{\mathrm{T}}\left(vec^{-1}\left\{adj\left\{-I_{n\times n}\otimes z_A(t) + \varphi(t)\,\Gamma^{\mathrm{T}}\otimes I_{n\times n}\right\} vec\left(z_B(t)\, h^{\mathrm{T}}\right)\right\}\right)\times \\ \times\Gamma^{-1} Y_{M^{-1}}(t)\, z_B(t) = \\ = h^{\mathrm{T}}\left(vec^{-1}\left\{adj\left\{-I_{n\times n}\otimes z_A(t) + \varphi(t)\,\Gamma^{\mathrm{T}}\otimes I_{n\times n}\right\} vec\left(z_B(t)\, h^{\mathrm{T}}\right)\right\}\right)\Gamma^{-1}\times \\ \times adj\left\{Y_M(t)\right\}\Delta_M(t)\, z_B(t) = \\ = h^{\mathrm{T}}\left(vec^{-1}\left\{adj\left\{-I_{n\times n}\otimes z_A(t) + \varphi(t)\,\Gamma^{\mathrm{T}}\otimes I_{n\times n}\right\} vec\left(z_B(t)\, h^{\mathrm{T}}\right)\right\}\right)\Gamma^{-1}\times \\ \times adj\left\{vec^{-1}\left(adj\left\{\overline{\Delta}_M(t)\right\}\overline{Y}_M(t)\right)\right\}\Delta_M(t)\, z_B(t) = \\ = h^{\mathrm{T}}\left(vec^{-1}\left\{adj\left\{-I_{n\times n}\otimes z_A(t) + \varphi(t)\,\Gamma^{\mathrm{T}}\otimes I_{n\times n}\right\} vec\left(z_B(t)\, h^{\mathrm{T}}\right)\right\}\right)\Gamma^{-1}\times \\ \times adj\left\{vec^{-1}\left(adj\left\{-I_{n\times n}\otimes z_A(t) + \varphi(t)\,\Gamma^{\mathrm{T}}\otimes I_{n\times n}\right\} vec\left(z_B(t)\, h^{\mathrm{T}}\right)\right)\right\}\times \\ \times\Delta_M(t)\, z_B(t) = \\ = h^{\mathrm{T}}\left(vec^{-1}\left\{adj\left\{-I_{n\times n}\otimes z_A(t) + \varphi(t)\,\Gamma^{\mathrm{T}}\otimes I_{n\times n}\right\} vec\left(z_B(t)\, h^{\mathrm{T}}\right)\right\}\right)\Gamma^{-1}\times \\ \times adj\left\{vec^{-1}\left(adj\left\{-I_{n\times n}\otimes z_A(t) + \varphi(t)\,\Gamma^{\mathrm{T}}\otimes I_{n\times n}\right\} vec\left(z_B(t)\, h^{\mathrm{T}}\right)\right)\right\}\times \\ \times\det\left\{\overline{\Delta}_M(t)\right\} z_B(t) = \\ = h^{\mathrm{T}}\left(vec^{-1}\left\{adj\left\{-I_{n\times n}\otimes z_A(t) + \varphi(t)\,\Gamma^{\mathrm{T}}\otimes I_{n\times n}\right\} vec\left(z_B(t)\, h^{\mathrm{T}}\right)\right\}\right)\Gamma^{-1}\times \\ \times adj\left\{vec^{-1}\left(adj\left\{-I_{n\times n}\otimes z_A(t) + \varphi(t)\,\Gamma^{\mathrm{T}}\otimes I_{n\times n}\right\} vec\left(z_B(t)\, h^{\mathrm{T}}\right)\right)\right\}\times \\ \times\det\left\{-I_{n\times n}\otimes z_A(t) + \varphi(t)\,\Gamma^{\mathrm{T}}\otimes I_{n\times n}\right\} z_B(t)\end{gathered} \tag{S16}$$

*where the operation* $vec^{-1}(.)$ *is feasible as the dimension of the matrix* $M$ *is known.*

*In their turn, the dependence of functions* $Y_x(t)$ *and* $Y_r(t)$ *from measurable signals* $z_A(t)$, $z_B(t)$ *and* $\varphi(t)$ *is written in explicit form as follows:*

$$\begin{gathered}Y_x := \left(adj\left\{\overline{\Delta}_x(t)\right\}\Delta_M(t)\, h\right)^{\mathrm{T}} = \\ = \left(adj\left\{Y_M^{\mathrm{T}}(t)\right\}\Delta_M(t)\, h\right)^{\mathrm{T}} = \\ = \left(adj\left\{\left(vec^{-1}\left(adj\left\{\overline{\Delta}_M(t)\right\}\overline{Y}_M(t)\right)\right)^{\mathrm{T}}\right\}\Delta_M(t)\, h\right)^{\mathrm{T}} = \\ = \begin{pmatrix} adj\left\{\left(vec^{-1}\left(adj\left\{-I_{n\times n}\otimes z_A(t) + \varphi(t)\,\Gamma^{\mathrm{T}}\otimes I_{n\times n}\right\} vec\left(z_B(t)\, h^{\mathrm{T}}\right)\right)\right)^{\mathrm{T}}\right\}\times \\ \times\Delta_M(t)\, h \end{pmatrix}^{\mathrm{T}} = \\ = \begin{pmatrix} adj\left\{\left(vec^{-1}\left(adj\left\{-I_{n\times n}\otimes z_A(t) + \varphi(t)\,\Gamma^{\mathrm{T}}\otimes I_{n\times n}\right\} vec\left(z_B(t)\, h^{\mathrm{T}}\right)\right)\right)^{\mathrm{T}}\right\}\times \\ \times\det\left\{\overline{\Delta}_M(t)\right\} h \end{pmatrix}^{\mathrm{T}} = \\ = \begin{pmatrix} adj\left\{\left(vec^{-1}\left(adj\left\{-I_{n\times n}\otimes z_A(t) + \varphi(t)\,\Gamma^{\mathrm{T}}\otimes I_{n\times n}\right\} vec\left(z_B(t)\, h^{\mathrm{T}}\right)\right)\right)^{\mathrm{T}}\right\}\times \\ \times\det\left\{-I_{n\times n}\otimes z_A(t) + \varphi(t)\,\Gamma^{\mathrm{T}}\otimes I_{n\times n}\right\} h \end{pmatrix}^{\mathrm{T}},\end{gathered} \tag{S17}$$

$$\begin{gathered}Y_r(t) := -\varphi(t)\,\Delta_M(t)\,\Delta_{M^{-1}}(t) = \\ = -\varphi(t)\det\left\{\overline{\Delta}_M(t)\right\}\Delta_{M^{-1}}(t) = \\ = -\varphi(t)\det\left\{-I_{n\times n}\otimes z_A(t) + \varphi(t)\,\Gamma^{\mathrm{T}}\otimes I_{n\times n}\right\}\Delta_{M^{-1}}(t) = \\ = -\varphi(t)\det\left\{-I_{n\times n}\otimes z_A(t) + \varphi(t)\,\Gamma^{\mathrm{T}}\otimes I_{n\times n}\right\}\det\left\{Y_M(t)\right\} = \\ = -\varphi(t)\det\left\{-I_{n\times n}\otimes z_A(t) + \varphi(t)\,\Gamma^{\mathrm{T}}\otimes I_{n\times n}\right\}\times \\ \times\det\left\{vec^{-1}\left(adj\left\{\overline{\Delta}_M(t)\right\}\overline{Y}_M(t)\right)\right\} = \\ = -\varphi(t)\det\left\{-I_{n\times n}\otimes z_A(t) + \varphi(t)\,\Gamma^{\mathrm{T}}\otimes I_{n\times n}\right\}\times \\ \times\det\left\{vec^{-1}\left(adj\left\{-I_{n\times n}\otimes z_A(t) + \varphi(t)\,\Gamma^{\mathrm{T}}\otimes I_{n\times n}\right\} vec\left(z_B(t)\, h^{\mathrm{T}}\right)\right)\right\}\end{gathered} \tag{S18}$$

*Hence, the equations* (S15)-(S18) *demonstrate that the regression (18) in the manuscript is implementable using only measurable signals (according to (17) in the manuscript)* $z_A(t)$, $z_B(t)$, $\varphi(t)$ *and known (according to the problem statement) matrices* $\Gamma, h$ *of the modal model (generator) (6) in the manuscript.*

## References


[1] A. Glushchenko, V. Petrov and K. Lastochkin, "I-DREM MRAC with Time-Varying Adaptation Rate and No A Priori Knowledge of Control Input Matrix Sign to Relax PE Condition", *in Proc. Eur. Control Conf.*, Rotterdam, Netherlands, 2021, pp. 2175-2180.
